# Supplementary material for: SAM: Self-adapting Mixture Prior to Dynamically Borrow Information from Historical Data in Clinical Trials
Source: arXiv:2305.12279 source file (2023-09-08)
Supplement: Supplementary file 1 [file SupplementMaterials-v8.pdf]

## Web Appendix

### A. Results for sensitivity analysis

#### A.1. Operating characteristics when the clinically significant difference $\delta = 0.15$

We studied the operating characteristics of self-adapting mixture (SAM) priors, in comparison to the fixed-weight mixture prior with  $\tilde{w} = 0.5$  (Mix50), power prior (PP), and commensurate prior (CP), when the clinically significant difference (CSD)  $\delta = 0.15$ . The endpoint is binary. We generated historical data  $D_h$  from *Bernoulli* ( $\theta_h$ ) with  $\theta_h = 0.4, 0.3, 0.2$ , and sample size  $n_h = 150$  for all three cases. When  $\theta_h = 0.4, 0.3$ , and  $0.2$ , the sample sizes for the control arm and treatment arm were set as  $n = 75, 75, 60$ , and  $n_t = 150, 150, 120$ , respectively. The sample sizes were chosen such that the power of the methods under comparison was mostly in the range of 70% to 90%. Figure S1 shows the relative bias and relative mean square error (RMSE), and Table S1 shows the type I error rate and power based on 2000 simulations.

**FIGURE S1** Relative bias (A) and Relative MSE (B) of the posterior mean using a SAM prior, a mixture prior with  $\tilde{w} = 0.5$  (Mix50), a power prior (PP), and a commensurate prior with a uniform prior (CP) for binary endpoints, with a non-informative prior (NP) as reference. The vertical dashed line represents  $\theta = \theta_h$ .

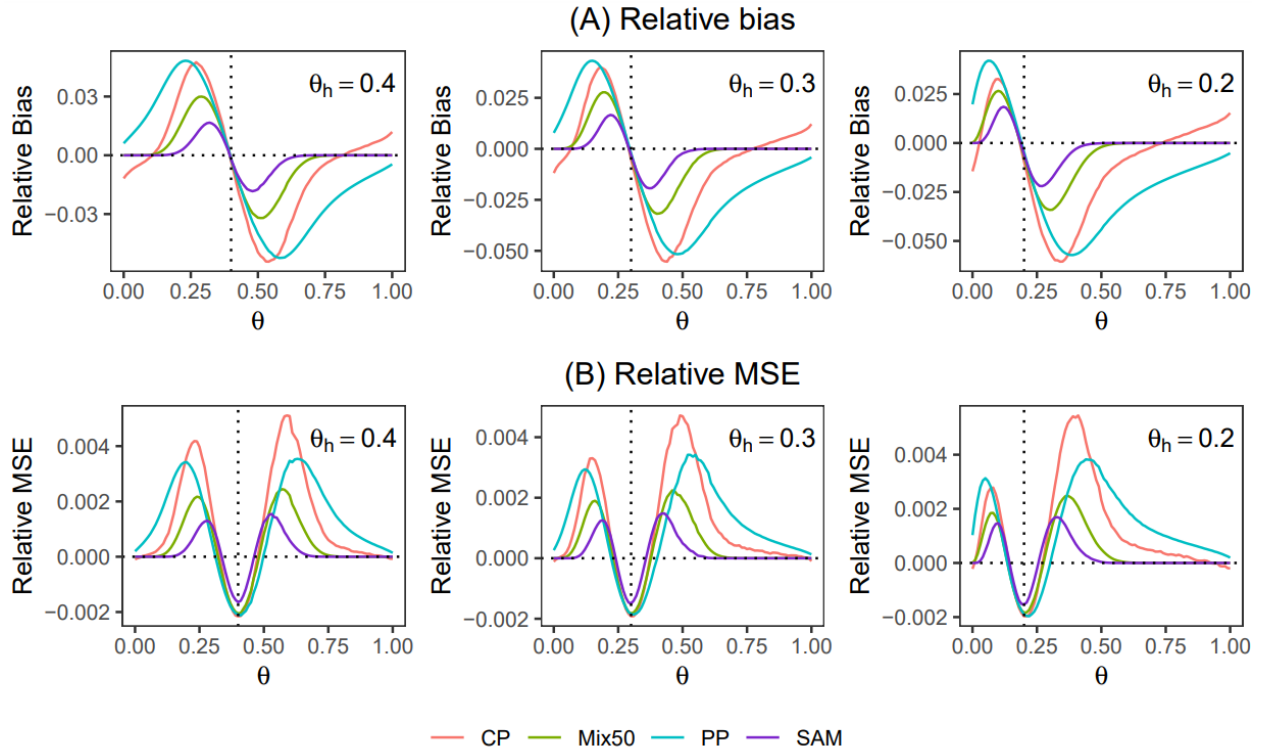

**TABLE S1** Simulation results for binary endpoints with  $\delta = 0.15$  using a noninformative prior (NP), a SAM prior, a mixture prior with  $\tilde{w} = 0.5$  (Mix50), a power prior (PP), and a commensurate prior with a uniform prior (CP).

| Scenario           | $\theta_c$ | $\theta_t$ | NP    | SAM   | Mix50 | PP    | CP    |
|--------------------|------------|------------|-------|-------|-------|-------|-------|
| <b>Case 1</b>      |            |            |       |       |       |       |       |
| <b>Congruent</b>   |            |            |       |       |       |       |       |
| 1.1*               | 0.4        | 0.4        | 0.050 | 0.050 | 0.050 | 0.051 | 0.050 |
| 1.2                | 0.4        | 0.55       | 0.683 | 0.876 | 0.904 | 0.905 | 0.904 |
| 1.3                | 0.41       | 0.56       | 0.678 | 0.874 | 0.911 | 0.912 | 0.906 |
| 1.4                | 0.38       | 0.53       | 0.698 | 0.875 | 0.883 | 0.877 | 0.856 |
| <b>Incongruent</b> |            |            |       |       |       |       |       |
| 1.5*               | 0.55       | 0.55       | 0.05  | 0.132 | 0.208 | 0.272 | 0.296 |
| 1.6*               | 0.6        | 0.6        | 0.052 | 0.076 | 0.138 | 0.267 | 0.219 |
| 1.7                | 0.25       | 0.4        | 0.735 | 0.712 | 0.588 | 0.54  | 0.452 |
| 1.8                | 0.2        | 0.35       | 0.768 | 0.788 | 0.682 | 0.529 | 0.478 |
| <b>Case 2</b>      |            |            |       |       |       |       |       |
| <b>Congruent</b>   |            |            |       |       |       |       |       |
| 2.1*               | 0.3        | 0.3        | 0.050 | 0.051 | 0.051 | 0.051 | 0.051 |
| 2.2                | 0.3        | 0.45       | 0.722 | 0.897 | 0.921 | 0.91  | 0.934 |
| 2.3                | 0.31       | 0.46       | 0.716 | 0.889 | 0.921 | 0.916 | 0.941 |
| 2.4                | 0.28       | 0.43       | 0.733 | 0.902 | 0.906 | 0.886 | 0.897 |
| <b>Incongruent</b> |            |            |       |       |       |       |       |
| 2.5*               | 0.45       | 0.45       | 0.05  | 0.12  | 0.173 | 0.27  | 0.288 |
| 2.6*               | 0.5        | 0.5        | 0.055 | 0.078 | 0.128 | 0.27  | 0.214 |
| 2.7                | 0.15       | 0.3        | 0.823 | 0.786 | 0.688 | 0.636 | 0.538 |
| 2.8                | 0.1        | 0.25       | 0.897 | 0.894 | 0.823 | 0.666 | 0.7   |
| <b>Case 3</b>      |            |            |       |       |       |       |       |
| <b>Congruent</b>   |            |            |       |       |       |       |       |
| 3.1*               | 0.2        | 0.2        | 0.051 | 0.050 | 0.051 | 0.051 | 0.051 |
| 3.2                | 0.2        | 0.35       | 0.693 | 0.882 | 0.906 | 0.927 | 0.916 |
| 3.3                | 0.21       | 0.36       | 0.691 | 0.886 | 0.906 | 0.93  | 0.926 |
| 3.4                | 0.18       | 0.33       | 0.706 | 0.904 | 0.902 | 0.904 | 0.88  |
| <b>Incongruent</b> |            |            |       |       |       |       |       |
| 3.5*               | 0.35       | 0.35       | 0.052 | 0.128 | 0.183 | 0.303 | 0.313 |
| 3.6*               | 0.4        | 0.4        | 0.053 | 0.082 | 0.122 | 0.298 | 0.22  |
| 3.7                | 0.05       | 0.2        | 0.892 | 0.888 | 0.765 | 0.702 | 0.662 |
| 3.8                | 0.03       | 0.18       | 0.952 | 0.945 | 0.936 | 0.737 | 0.806 |

\*Indicates type I error.

### A.2. The mixture weight in the SAM prior in relation to clinically significant difference $\delta$

In order to evaluate the sensitivity of the SAM prior, we investigated the change of the mixture weight  $w$  in relation to the CSD, for both binary and continuous endpoints. Our simulation setup closely mirrors the one described in the main simulation (Section 3.1) of the paper. For the binary case, we utilized a grid of  $\delta$  values ranging from 0.01 to 0.15, with a step size of 0.02. Meanwhile, the continuous case used a grid of  $\delta$  values  $\{0.01, 0.2, 0.35, 0.5, 0.65, 0.8, 1\}\sigma$ , where  $\sigma = 3$ , consistent with the main text simulation setting. Figure S2 illustrates the changes in mixture weights associated with varying degrees of prior-data conflicts. Our findings suggest that the mixture weights are concentrated within the CSD, and decrease significantly as the level of prior-data conflicts increases.

**FIGURE S2** Mixture weight of the SAM prior under different degrees of prior-data conflict (i.e.,  $\theta - \theta_h$ ) and CSD (i.e.,  $\delta$ ) for binary and continuous endpoints. The vertical line stands for  $\theta = \theta_h$ .

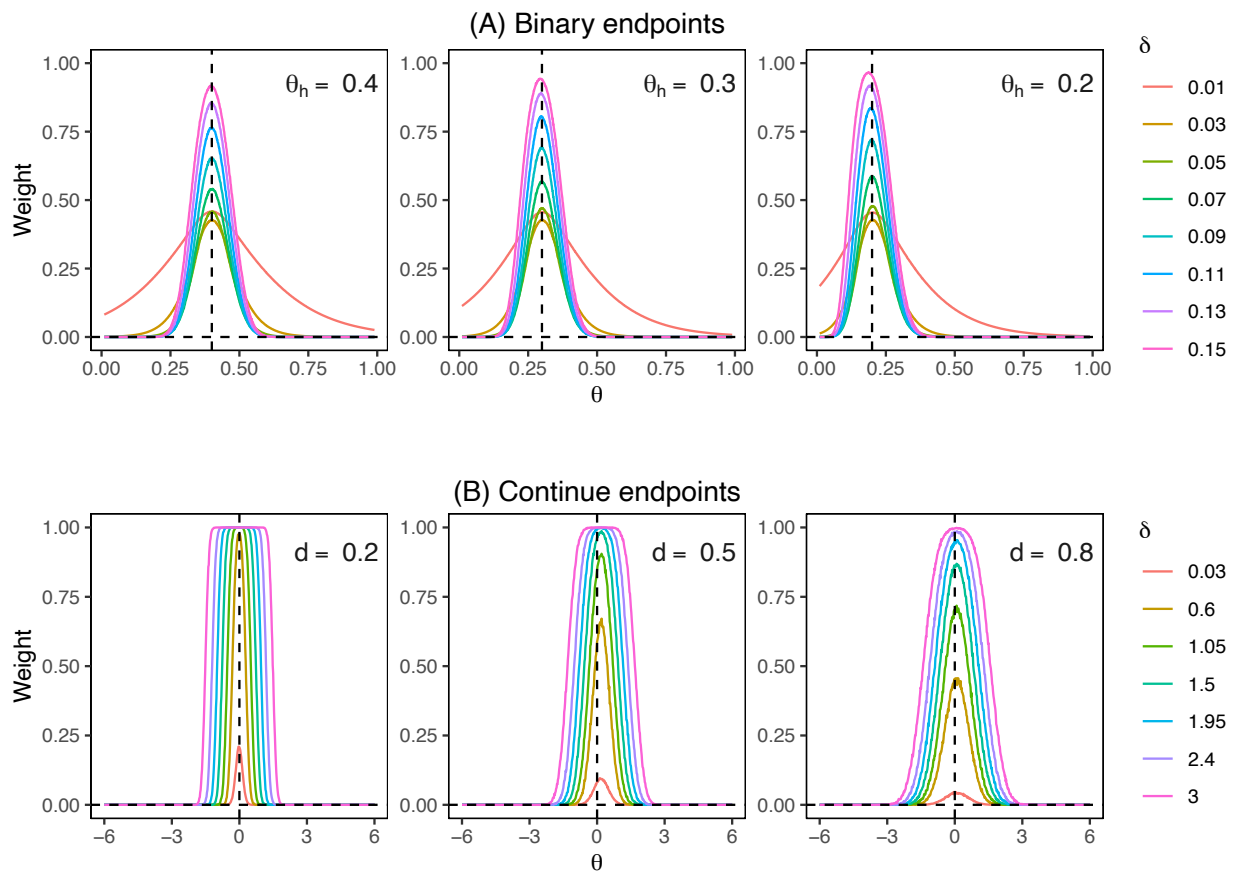

## B. Operating characteristics of fixed-weight mixture priors using bimodal prior

Another approach to account for  $H_1$  and CSD is to assign a bimodal prior for  $\pi_0(\theta)$  in the fixed-weight mixture prior, with two modes centered at  $\theta_h - \delta$  and  $\theta_h + \delta$ . We considered two bimodal priors, including the inverse moment (iMOM) prior (Johnson and Rossell, 2010) and a mixture of beta/normal distributions (Figure S3). Specifically, we investigated the bimodal beta/normal prior with  $\tilde{w} = 0.5$  (rMAP50) for binary and continuous endpoints, respectively, and the non-local inverse moment (iMOM) prior with  $\tilde{w} = 0.5$  (iMAP50) as  $\pi_0(\theta)$ . The non-local iMOM balances the convergence rates of evidence gain with null and alternative hypotheses as the sample size increases. The iMOM prior is defined as follows:

$$\pi_I(\theta; \theta_0, k, v, \tau) = \frac{k\tau^v}{\Gamma(v/2k)} [(\theta - \theta_0)^2]^{-\frac{v+1}{2}} \exp \left\{ - \left[ \left( \frac{\theta - \theta_0}{\tau} \right)^2 \right]^{-k} \right\}.$$

This density function has two modes at

$$\hat{\theta} = \theta_0 \pm \tau \left[ \frac{2k}{v+1} \right]^{1/2k}.$$

We used  $k = 1$  and  $v = 2$  to back-solve for the corresponding  $\tau$  values, ensuring that the modes of the bimodal priors are centered at  $\theta_h - \delta$  and  $\theta_h + \delta$  for a given  $\delta$ . We then evaluated the performance of the two bimodal prior approaches and compared them to SAM priors. The simulation setup was the same as the main simulation described in Section 3.1 of the main text, and we obtained the posterior mean estimates of  $\theta$  using importance sampling.

Simulation results showed that bimodal priors do not perform as well as the SAM prior, as evidenced by larger relative bias and mean squared errors (MSEs) as prior-data conflict increases (see Figures S4-5). The poor performance of bimodal priors can be attributed to the fact that the probability mass outside the two modes,  $\theta_h - \delta$  and  $\theta_h + \delta$ , is low. This resulted in the likelihood of historical data dominating the posterior inference outside this range, leading to substantial bias in the estimates.

**FIGURE S3** An example of a bimodal beta distribution (orange line) and an iMOM distribution (pink line). The vertical dashed line represents  $\theta = \theta_h \pm \delta$  with  $\delta = 0.1$ .

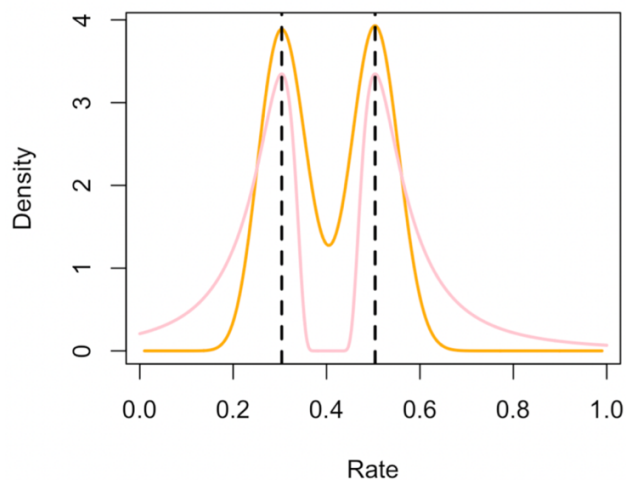

**FIGURE S4** Relative bias (A) and Relative MSE (B) of the posterior mean using a SAM prior, a mixture bimodal beta prior with  $\tilde{w} = 0.5$  (rMix50), the iMOM prior with  $\tilde{w} = 0.5$  (iMix50) for binary endpoints, with a non-informative prior (NP) as reference. The vertical dashed line represents  $\theta = \theta_h$ .

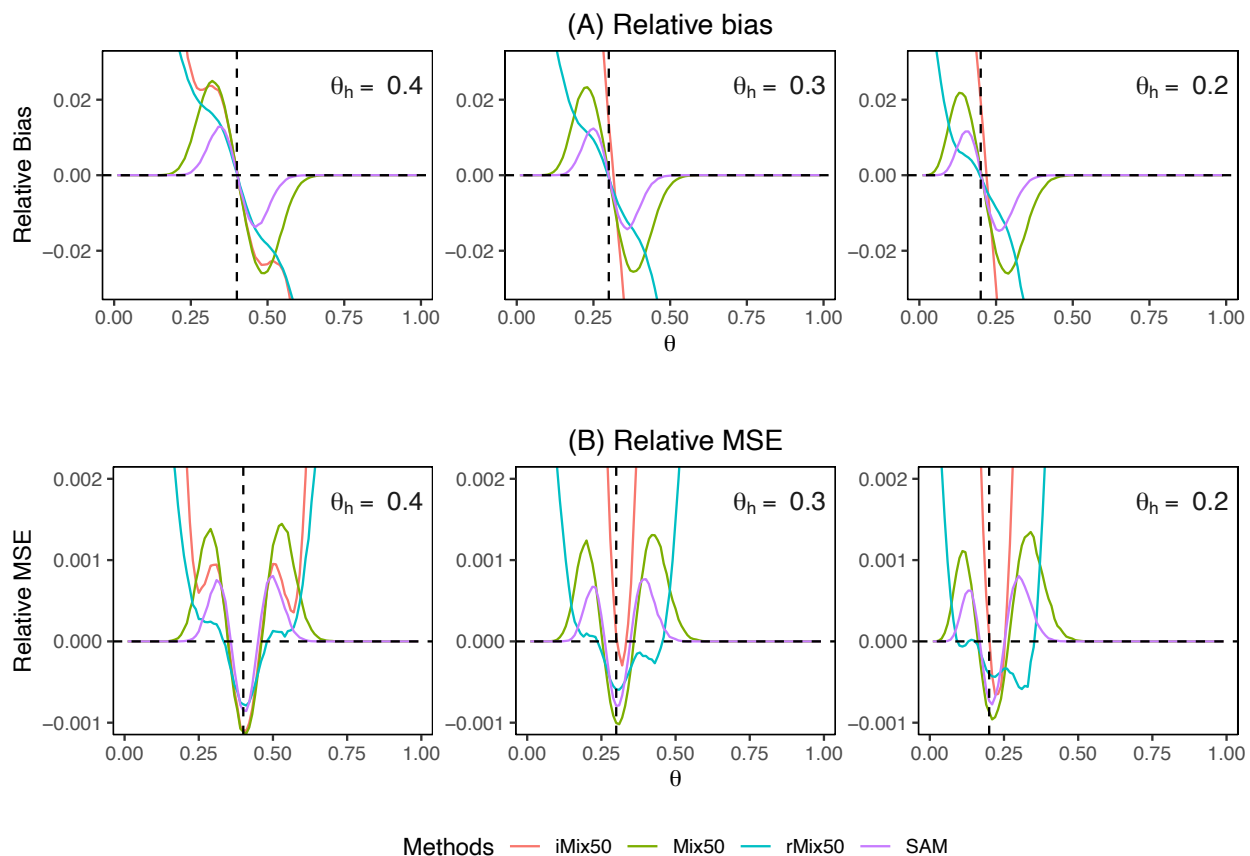

**FIGURE S5** Relative bias (A) and Relative MSE (B) of the posterior mean using a SAM prior, a mixture bimodal normal prior with  $\tilde{w} = 0.5$  (rMix50), the iMOM prior with  $\tilde{w} = 0.5$  (iMix50) for continuous endpoints, with a non-informative prior (NP) as reference. The vertical dashed line represents  $\theta = \theta_h$ .

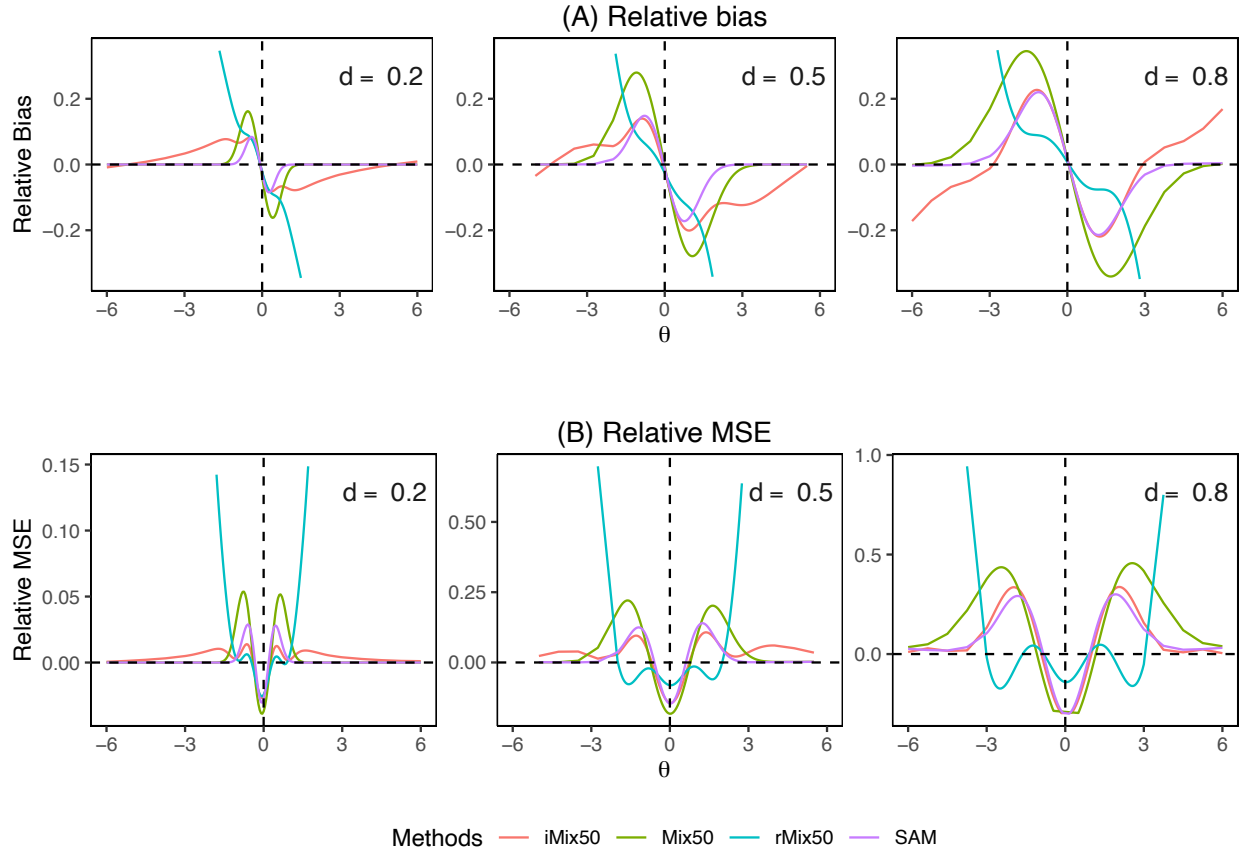

### C. SAM priors for survival endpoints

In this section, we introduce how to apply SAM prior to survival endpoints. Assume historical data  $D_h$  consisting of  $T_{h1}, T_{h2}, \dots, T_{hn_h} \sim \exp(\lambda_h)$ , subject to non-informative right censoring  $C_{h1}, C_{h2}, \dots, C_{hn_h}$ . Let  $U_{hi} = \min(C_{hi}, t_{hi})$  denote the observed time, and  $\delta_{hi} = I(T_{hi} < C_{hi})$  denote the censoring indicator. Let  $\lambda$  denote the hazard of the current trial control. Given a non-informative gamma prior,  $\lambda \sim \text{Gamma}(\alpha, \beta)$ , e.g.,  $\alpha = \beta = 0.1$ , the informative prior that incorporates historical information is given by:

$$\pi_1(\lambda) = \text{Gamma}(\alpha + r_h, \beta + Q_h),$$

where  $r_h = \sum_{i=1}^{n_h} \delta_{hi}$  and  $Q_h = \sum_{i=1}^{n_h} u_{hi}$  represent the number of events and the total observed time, respectively. The SAM prior arises as

$$\pi_{sam}(\lambda) = w \text{Gamma}(\alpha + r_h, \beta + Q_h) + (1 - w) \text{Gamma}(\alpha, \beta),$$

where  $w = \frac{R}{1+R}$  with

$$R = \frac{\hat{\lambda}_h^r \exp\{-\hat{\lambda}_h Q\}}{\max\{(\hat{\lambda}_h - \delta)^r \exp\{-(\hat{\lambda}_h - \delta)Q\}, (\hat{\lambda}_h + \delta)^r \exp\{-(\hat{\lambda}_h + \delta)Q\}\}},$$

where  $\hat{\lambda}_h = (\alpha + r_h)/(\beta + Q_h)$ . Owing to its conjugacy, given  $\pi_{sam}(\lambda)$  and trial data  $D$ , the posterior of  $\lambda$  is given by

$$p(\lambda|D, D_h) = w^* \text{Gamma}(\alpha + r_h + r, \beta + Q_h + Q) + (1 - w^*) \text{Gamma}(\alpha + r, \beta + Q),$$

where  $w^*$  is the re-weighted  $w$  by the posterior normalizing constant associated with each mixture component, given by

$$\begin{aligned} w^* &= \frac{w z_1}{w z_1 + w z_0}, \\ z_0 &= \frac{\beta^\alpha \Gamma(\alpha + r)}{\Gamma(\alpha)(\beta + Q)^{\alpha+r}}, \\ z_1 &= \frac{(\beta + Q_h)^\alpha \Gamma(\alpha + r + r_h)}{\Gamma(\alpha + r_h)(\beta + Q + Q_h)^{\alpha+r+r_h}}. \end{aligned}$$

A similar approach can be applied to a more flexible piecewise exponential model.

We conducted a simulation study to evaluate the operating characteristics of the SAM prior for survival endpoints. We considered three hazards for  $D_h$ , i.e.,  $\lambda_h = 0.5, 1$ , and  $2$ , with the sample size  $n_h = 100, 60$ , and  $30$ , respectively, and simulated control arm data  $D$  with the sample size  $n = 50, 30$ , and  $12$ , respectively. The sample sizes were chosen such that the power of the methods under comparison is mostly in the range of 70% to 90%. For each of the three values of  $\lambda_h$ , we varied the hazard of the current control (i.e.,  $\lambda$ ) to generate different degrees of prior-data conflict, and set  $\delta = 0.1, 0.2$ , and  $0.4$  for the three cases. We conducted 2000 simulations for each configuration. We compared the SAM prior with Mix50.

We found that the SAM prior has uniformly smaller relative biases and mean squared errors (MSEs) than Mix50 (Figure S6). Furthermore, Table S2 displays the type I error and power when  $\lambda_h = 1$ ,

$n = n_h = 50$ , and  $n_t = 100$ , which demonstrates that the SAM prior provides more power gain than Mix50 while maintaining reasonable type I error rates.

**FIGURE S6** Relative bias (A) and Relative MSE (B) of the posterior mean using a SAM prior, a mixture prior with  $\tilde{w} = 0.5$  (Mix50) for survival endpoints, with a non-informative prior (NP) as reference. The vertical dashed line represents  $\lambda = \lambda_h$ .

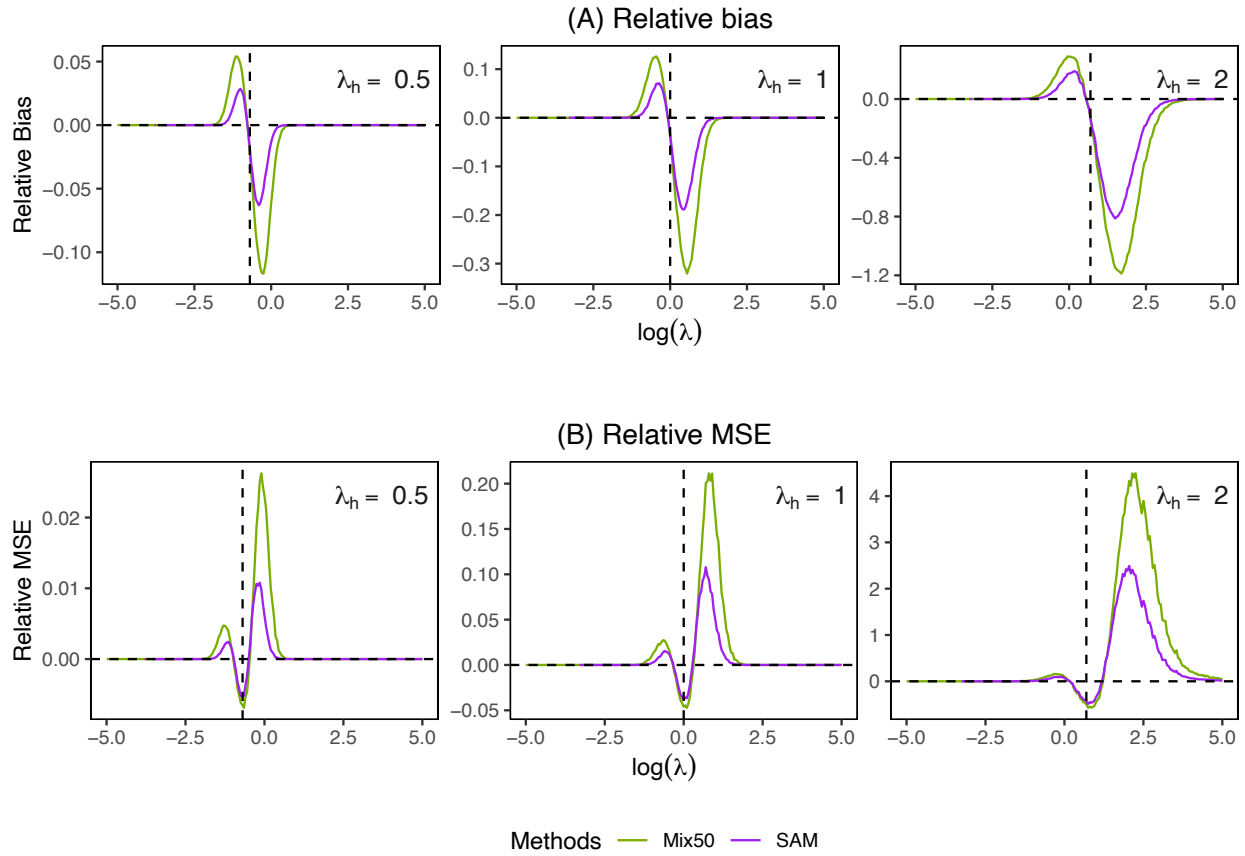

**TABLE S2** Simulation results for survival endpoints with  $\delta = 0.4$  using a noninformative prior (NP), a SAM prior, a mixture prior with  $\tilde{w} = 0.5$  (Mix50).

| Scenario           | $\lambda_c$ | $\lambda_t$ | NP    | SAM   | Mix50 |
|--------------------|-------------|-------------|-------|-------|-------|
| <b>Congruent</b>   |             |             |       |       |       |
| 1*                 | 1.00        | 1.00        | 0.052 | 0.051 | 0.052 |
| 2                  | 1.00        | 1.60        | 0.808 | 0.974 | 0.720 |
| 3                  | 0.90        | 1.40        | 0.782 | 0.876 | 0.596 |
| 4                  | 0.95        | 1.45        | 0.739 | 0.875 | 0.508 |
| <b>Incongruent</b> |             |             |       |       |       |
| 5*                 | 0.70        | 0.70        | 0.053 | 0.067 | 0.002 |
| 6*                 | 1.30        | 1.30        | 0.052 | 0.154 | 0.172 |
| 7                  | 0.50        | 1.00        | 0.967 | 0.984 | 0.867 |
| 8                  | 0.70        | 1.20        | 0.887 | 0.886 | 0.434 |

\*Indicates type I error.

#### D. Ankylosing spondylitis trial data and sensitivity analysis.

Table S3 displays historical data on the placebo from 9 studies. Notably, the study by Baeten (2013) has a small sample size ( $n=6$ ), which raises concerns about its inclusion in the analysis. As a sensitivity analysis, we redid the analysis by excluding the dataset from Baeten (2013). The resulting MAP prior from the remaining datasets is  $\pi_1(\theta) = 0.64\text{Beta}(39.9, 71.6) + 0.35\text{Beta}(7.2, 12.4)$ , which is very similar to that obtained when Baeten (2013) was included, i.e.,  $\pi_1(\theta) = 0.63\text{Beta}(42.5, 77.2) + 0.37\text{Beta}(7.2, 12.4)$ . The mean of the resulting MAP prior is  $\hat{\theta}_h = 0.362$ . Table S4 displays the type I error and power, in comparison with the robust MAP prior with  $\tilde{w} = 0.5$  (Mix50) and 0.9 (Mix90), after excluding Baeten (2013). Additionally, Figure S7 shows the relative bias and RMSE of SAM, Mix50, and Mix90 after excluding Baeten (2013). The findings are comparable to those obtained using all datasets, as shown in Figure 4 and Table 3 in the main text.

**TABLE S3** Historical data of placebo arms from nine clinical trials with ASAS20 response as the primary endpoint.

| Author/Year           | Events | Total |
|-----------------------|--------|-------|
| Baeten (2013)         | 1      | 6     |
| Deodhar (2016)        | 35     | 122   |
| Deodhar (2019)        | 31     | 104   |
| Erdes (2019)          | 10     | 23    |
| Huang (2019)          | 56     | 153   |
| Kivitz (2018)         | 55     | 117   |
| Pavelka (2017)        | 28     | 76    |
| Sieper (2017)         | 21     | 74    |
| van der Heijde (2018) | 35     | 87    |

**TABLE S4** Type I error and power of the SAM prior, in comparison with the robust MAP prior with  $\tilde{w} = 0.5$  (Mix50) and 0.9 (Mix90), for ankylosing spondylitis trial with the dataset from Baeten (2013) excluded.

| Scenario           | $\theta_c$ | $\theta_t$ | NP    | SAM   | Mix50 | Mix90 |
|--------------------|------------|------------|-------|-------|-------|-------|
| <b>Congruent</b>   |            |            |       |       |       |       |
| 1*                 | 0.36       | 0.36       | 0.050 | 0.052 | 0.051 | 0.052 |
| 2                  | 0.36       | 0.56       | 0.620 | 0.819 | 0.817 | 0.864 |
| 3                  | 0.37       | 0.57       | 0.644 | 0.806 | 0.803 | 0.880 |
| 4                  | 0.34       | 0.54       | 0.634 | 0.788 | 0.786 | 0.850 |
| <b>Incongruent</b> |            |            |       |       |       |       |
| 5*                 | 0.56       | 0.56       | 0.06  | 0.112 | 0.142 | 0.269 |
| 6*                 | 0.61       | 0.61       | 0.056 | 0.083 | 0.119 | 0.240 |
| 7                  | 0.16       | 0.36       | 0.725 | 0.697 | 0.577 | 0.443 |
| 8                  | 0.11       | 0.31       | 0.760 | 0.766 | 0.651 | 0.469 |

**FIGURE S7** (A) Relative bias and (B) relative mean square error (RMSE) for the posterior mean estimate of  $\theta$  for the SAM prior and robust MAP prior with  $\tilde{w} = 0.5$  (Mix50) and 0.9 (Mix90) in ankylosing spondylitis trial with the dataset from Baeten (2013) excluded. Panel (C) depicts how the weight of the SAM prior self-adapts to prior-data conflict (i.e.,  $\theta - \theta_h$ ). The vertical dotted line indicates  $\theta = \theta_h$ .

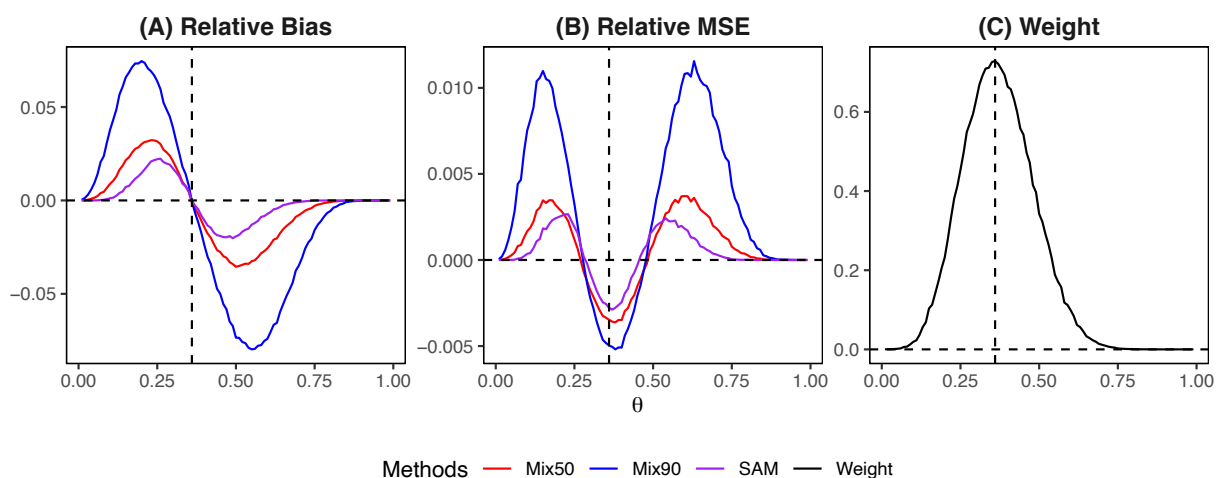

## E. Cutoff $C$ used in simulations

**TABLE S5** The calibrated values of cutoff  $C$  in simulations and ankylosing spondylitis trial.

| Scenario                                                | NP    | SAM   | Mix50 | PP    | CP    | SAM   | Mix90 |
|---------------------------------------------------------|-------|-------|-------|-------|-------|-------|-------|
| <b>binary endpoints with <math>\delta = 0.1</math></b>  |       |       |       |       |       |       |       |
| Case 1                                                  | 0.949 | 0.932 | 0.925 | 0.922 | 0.94  | 0.928 | -     |
| Case 2                                                  | 0.949 | 0.937 | 0.925 | 0.923 | 0.944 | 0.934 | -     |
| Case 3                                                  | 0.943 | 0.939 | 0.922 | 0.922 | 0.947 | 0.936 | -     |
| <b>normal endpoints</b>                                 |       |       |       |       |       |       |       |
| Case 1                                                  | 0.948 | 0.933 | 0.920 | 0.919 | 0.926 | 0.930 | -     |
| Case 2                                                  | 0.946 | 0.936 | 0.925 | 0.918 | 0.928 | 0.933 | -     |
| Case 3                                                  | 0.953 | 0.947 | 0.934 | 0.922 | 0.937 | 0.943 | -     |
| <b>binary endpoints with <math>\delta = 0.15</math></b> |       |       |       |       |       |       |       |
| Case 1                                                  | 0.949 | 0.938 | 0.922 | 0.922 | 0.947 | -     | -     |
| Case 2                                                  | 0.945 | 0.938 | 0.923 | 0.922 | 0.945 | -     | -     |
| Case 3                                                  | 0.945 | 0.937 | 0.928 | 0.917 | 0.950 | -     | -     |
| <b>survival endpoints</b>                               |       |       |       |       |       |       |       |
|                                                         | 0.952 | 0.910 | 0.986 | -     | -     | -     | -     |
| <b>Ankylosing spondylitis trial</b>                     |       |       |       |       |       |       |       |
| Full datasets                                           | 0.945 | 0.944 | 0.931 | -     | -     | -     | 0.923 |
| Exclude Baeten (2013)                                   | 0.945 | 0.943 | 0.933 | -     | -     | -     | 0.930 |

## F. Reference

- Baeten D, Baraliakos X, Braun J, Sieper J, Emery P, van der Heijde D, McInnes I, van Laar JM, Landewé R, Wordsworth P, Wollenhaupt J, Kellner H, Paramarta J, Wei J, Brachat A, Bek S, Laurent D, Li Y, Wang YA, Bertolino AP, Gsteiger S, Wright AM, Hueber W. (2013) Antiinterleukin-17A monoclonal antibody secukinumab in treatment of ankylosing spondylitis: a randomised, double-blind, placebo-controlled trial. *Lancet* 382,1705–1713.
- Deodhar AA, Dougados M, Baeten DL, Cheng-Chung Wei J, Geusens P, Readie A, Richards HB, Martin R, Porter B. (2016) Effect of secukinumab on patient-reported outcomes in patients with active ankylosing spondylitis a phase III randomized trial (MEASURE 1). *Arthritis and Rheumatology*, 68, 2901–2910.
- Deodhar A, Poddubnyy D, Pacheco-Tena C, Salvarani C, Lespessailles E, Rahman P, Järvinen P, Sanchez-Burson J, Gaffney K, Lee EB, Krishnan E, Santisteban S, Li X, Zhao F, Carlier H, Reveille JD, COAST-W Study Group. (2019) Efficacy and safety of ixekizumab in the treatment of radiographic axial spondyloarthritis: sixteen-week results from a phase III randomized, double-blind, placebo-controlled trial in patients with prior inadequate response to or intolerance of tumor necrosis factor inhibitors. *Arthritis and Rheumatology*, 71, 599–611.
- Erdes S, Nasonov E, Kunder E et al. (2020) Primary efficacy of netakimab, a novel interleukin-17 inhibitor, in the treatment of active ankylosing spondylitis in adults. *Clin Exp Rheumatol*, 38, 27-34.
- Huang, F., F. Sun, W. Wan, et al. (2019) Secukinumab provides rapid and significant improvement in the signs and symptoms of ankylosing spondylitis: primary (16-week) results from a phase 3 China-centric study, measure 5. *Annals of the Rheumatic Diseases*, 78, 894-895.
- Johnson, V., and Rossell, D. (2010) On the use of non-local prior densities in Bayesian hypothesis tests. *Journal of the Royal Statistical Society: Series B (Statistical Methodology)*, 72, 143-170.
- Kivitz AJ, Wagner U, Dokoupilova E, Supronik J, Martin R, Tallozy Z, Richards HB, Porter B. (2018) Efficacy and safety of secukinumab 150 mg with and without loading regimen in ankylosing spondylitis: 104-week results from MEASURE 4 study. *Rheumatology and Therapy*, 5, 447–462.
- Pavelka, K., A. Kivitz, E. Dokoupilova, et al (2017) Efficacy, safety, and tolerability of secukinumab in patients with active ankylosing spondylitis: a randomized, double-blind phase 3 study, MEASURE 3. *Arthritis Research and Therapy*, 19 (1), 285.

Sieper J, Deodhar A, Marzo-Ortega H, Aelion JA, Blanco R, JuiCheng T, Andersson M, Porter B, Richards HB, MEASURE 2 Study Group. (2017) Secukinumab efficacy in anti-TNF-naïve and anti-TNF-experienced subjects with active ankylosing spondylitis: results from the MEASURE 2 study. *Ann Rheum Dis*, 76, 571–575.

van der Heijde D, Cheng-Chung Wei J, Dougados M, Mease P, Deodhar A, Maksymowych WP, van den Bosch F, Sieper J, Tomita T, Landewé R, Zhao F, Krishnan E, Adams DH, Pangallo B, Carlier H, COAST-V study group. (2018) Ixekizumab, an interleukin-17A antagonist in the treatment of ankylosing spondylitis or radiographic axial spondyloarthritis in patients previously untreated with biological disease-modifying anti-rheumatic drugs (COAST-V): 16 week results of a phase 3 randomised, double-blind, activecontrolled and placebo-controlled trial. *Lancet*, 392, 2441–2451.
